# Supplementary material for: Moving perturbation in a one-dimensional Fermi gas
Source: arXiv:1312.0810 source file (2014-12-02)
Supplement: Supplementary file 1 [file supplemental.pdf]

# Moving perturbation in a one-dimensional Fermi gas - Supplemental material

## Wave front velocities

The velocities of the density wave fronts in Table I of the main text are extracted by making a linear fit  $x(t) = v_{\text{w.f.}}^\uparrow t + x_0$  to the approximate edge of the wave, as shown in Fig. S1. The edge points are obtained as the points where the density change reaches 20 % of the minimum of each time step within a time interval where the propagation is linear. Error bars for the coefficients  $v_{\text{w.f.}}^\uparrow$  are obtained as the 95 % confidence intervals, and the largest error is quoted in the text above Table I.

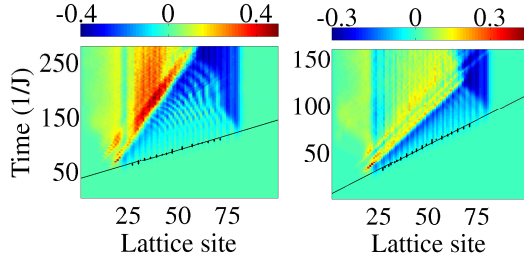

FIG. S1: (Color online). The density difference  $n_{i\uparrow}(t) - n_{i\uparrow}(0)$  as in Fig. 2. Black dots mark the wave front edge where the density change is 20 % of the minimum and a linear fit to them is shown as a black line.

## The non-interacting system

Comparison to the non-interacting case reveals a clear difference in the particle kinetics. For non-interacting particles, the phase difference is more irregular than in the interacting case, as shown in Fig. S2. This is due to the increased movement of particles, as seen in the density profiles of Fig. S3: In the fast regime, there is a larger deviation from the ground state than in the interacting case. For slow perturbations, a wave front of hole excitations propagates with the single-particle velocity (Table I of the main text) and is seen as a small reduction of density in the right edge of the cloud at  $t = 60 \frac{1}{J}$ . Therefore, compared to the interacting case of Fig. 4 of the main text, the coherence in the phase is broken earlier in the whole particle cloud. We have used a single-doublon model to describe the phase imprinted on the wave function in the high-velocity regime. Apart from the irregularities, this description extends to the limit of no interactions. For two non-interacting particles with a wavefunction  $|\psi(t)\rangle = |\psi_\uparrow(t)\rangle |\psi_\downarrow(t)\rangle = [\sum_i \alpha_i(t) |\uparrow_i\rangle][\sum_j \beta_j(t) |\downarrow_j\rangle]$ , where  $|\sigma_i\rangle = |0, 0, \dots, \sigma_i, 0, \dots, 0\rangle$ , the pair correlation function is  $\langle \psi | c_{i\uparrow}^\dagger c_{j\downarrow}^\dagger c_{j\downarrow} c_{i\uparrow} | \psi \rangle = e^{-i\Delta\phi} |\alpha_i| |\beta_i| |\alpha_j| |\beta_j|$ , giving the same phase factor as for the single doublon. For  $v = 0.5 J$ , the densities are closer to the equilibrium ones than in the interacting case. The small oscillations that remain

in the distributions of Fig. S3 are Friedel oscillations due to the finite size of the system.

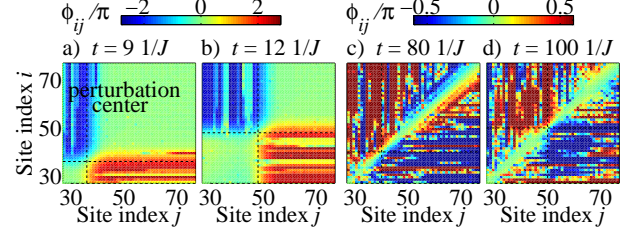

FIG. S2: (Color online). The phase  $\phi_{ij}$  at different time steps for  $v = 4 J$  (a, b) and  $v = 0.5 J$  (c, d) of the Gaussian potential well with  $V_0 = -2 J$ , for  $U = 0 J$ .

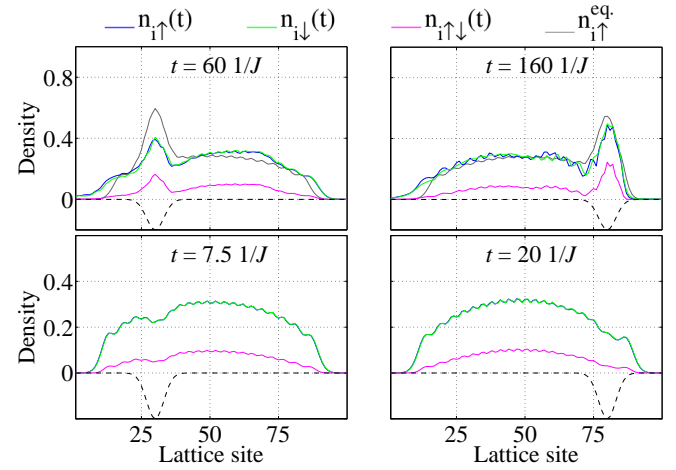

FIG. S3: (Color online). The density distributions at different time steps as in Fig. 1 of the main text, for  $U = 0 J$ . The first row shows a slow Gaussian well ( $V_0 = 2 J$ ) with  $v = 0.5 J$  and the second row a fast one with  $v = 4 J$ .

A striking difference between the interacting and non-interacting cases is observed when considering the decay of the correlations. The decay of  $|C_{ij}|$  for  $U = 0$  is shown on logarithmic scale in Fig. S4. Since in the non-interacting case, there are no nontrivial pair correlations in the ground state, the decay law of  $|C_{ij}|$  does not change when the system is perturbed. In other words, the velocity of the perturbation does not essentially affect the correlations. In contrast, in the interacting system, a slow perturbation reduces  $|C_{ij}|$  to the same decay law as in the non-interacting case, indicating that the initial nontrivial pair correlations are broken. Thus the correlations are preserved in the fast and destroyed in the slow perturbation regimes. The drastic difference between the interacting and non-interacting cases highlights the role and fate of pair correlations in the presence of a moving perturbation.

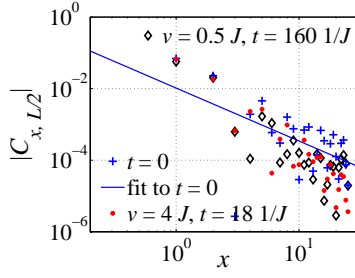

FIG. S4: (Color online). The pair correlation  $|C_{x > \frac{L}{2}, \frac{L}{2}}|$  for  $U = 0$  shown as in Fig. 3 of the main text. A fit  $f(x) = kx + a$  to the ground state correlation gives the coefficients  $k = -1.5 \pm 0.9$  and  $a = -5 \pm 2$ .

### The perturbations in momentum-frequency space

The moving wave-packet perturbation probes certain regions of the excitation spectrum. These regions are given by the Fourier transforms  $\tilde{V}(k, \omega)$  of the perturbing potentials. In the case of a Gaussian function, the Fourier transform is

$$\begin{aligned} \tilde{V}_G(k, \omega) &= \int_0^T \left[ \int_{-\infty}^{\infty} V_0 e^{-\frac{(x-vt)^2}{2\sigma^2}} e^{-ikx} dx \right] e^{-i\omega t} dt \\ &= 4\sqrt{2\pi}\sigma V_0 e^{-\frac{1}{2}\sigma^2 k^2} e^{-iaT} T \text{sinc}(aT), \end{aligned}$$

where  $a = \frac{1}{2}(vk + \omega)$ . Due to the finite size of the system, the time integral is over a finite period. The space integral

can be approximated to infinity for fast-decaying perturbations. For the Lorentzian perturbation, the Fourier transform is  $\tilde{V}_L(k, \omega) = 4\pi e^{-\gamma|k|} e^{-iaT} T \text{sinc}(aT)$ . The functions have a symmetric distribution around  $k = 0$  in momentum space and oscillations around the  $\omega = -vk$  peak in the frequency part, as shown in Fig. S5. The perturbations can therefore excite modes with various velocities. In an infinite system, the possible excitations are limited since the frequency part is a delta function,  $\lim_{T \rightarrow \infty} T \text{sinc}(aT) = \delta(a)$ .

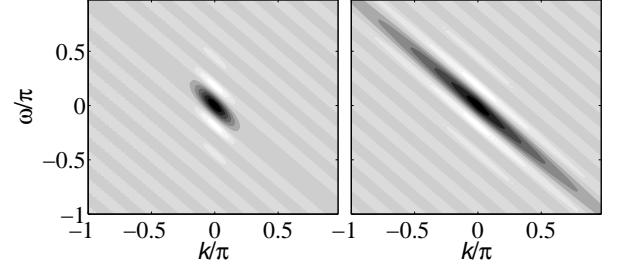

FIG. S5: Contours of the Fourier transforms  $|\tilde{V}_G(k, \omega)|$  (left) and  $|\tilde{V}_L(k, \omega)|$  (right) for  $v = 1 J$ , where black denotes the maximum value and white the minimum. A small value of  $T$  ( $T = 5 \frac{1}{J}$ ) is used for plotting in order to make the oscillations in the frequency part visible.
